# Supplementary material for: A Risk-Managed Steady-State Analysis to Assess the Impact of Power Grid Uncertainties
Source: arXiv:2111.10290 source file (2022-11-08)
Supplement: Supplementary file 1 [file appendix.tex]

\appendix

\subsection{Characteristic Functions}

The characteristic function $\phi_{X}(t)$ of the random variable $X$ is for $t \in \mathbb{R}$ given by \cite{Koski-2017}

\begin{equation}
        \phi_{X}(t) = \mathbb{E}[e^{jt\mathbf{x}}] = \Bigg\{ \begin{matrix} \sum_{k=-\infty}^{\infty} \exp(jtx_k) p_{X}(x_k)  & \textnormal{discrete r.v.} \\ \\  \int_{-\infty}^{\infty}\exp(jtx) f_{X}(x) dx & \textnormal{continuous r.v.}\end{matrix}
        \label{eq:def_char_fun}
\end{equation}

The characteristic function exists for any random variable \cite{Koski-2017}.

The characteristic function of $a + bX$ where $a$ and $b$ are real numbers is \cite{Koski-2017},
\begin{equation}
    \phi_{a + bX}(t) = \exp(jat)\phi_{X}(bt)
    \label{eq:affine_char_fun}
\end{equation}

This affine transformation property also applies to multivariate distributions as well \cite{Koski-2017}.

\subsection{Characteristic Function of Normal Distribution}
$X$ is a normal random variable. The characteristic function of a normally distributed random variable is \cite{Koski-2017}
\begin{equation}
    \phi_{X}(t) = E[e^{jtX}] = \exp(jt\mu - \frac{\sigma^2t^2}{2})
    \label{eq:normal_char_fun}
\end{equation}
where $\mu$ is the mean of the random variable, $\sigma$ is the standard deviation, and $\sigma^2$ is the variance.

\subsection{Characteristic Function Multivariate Normal Distribution}
$\mathbf{X}$ has a multivariate normal distribution with mean vector $\mu$ and covariance matrix $\mathbf{\Sigma}$, expressed as $\mathbf{X} \in N(\mu, \Sigma)$, if and only if the characteristic function is \cite{Koski-2017}

\begin{equation}
    \phi_{\mathbf{X}}(\mathbf{t}) = \exp(j\mathbf{t}^T\mu - \frac{1}{2}\mathbf{t}^T\Sigma\mathbf{t})
    \label{eq:mvn_char_fun}
\end{equation}

\subsection{Worst-Case Performance Derivation}\label{appendix}
Using the definition of characteristic functions \eqref{eq:def_char_fun}, the characteristic function for multivariate normal distributions \eqref{eq:mvn_char_fun}, and the affine transformation property of characteristic functions \eqref{eq:affine_char_fun} we can find that

\begin{align}
    \phi_{c_i}(t) &= \mathbb{E}[e^{jtc_i}] \\
    &= \mathbb{E}[e^{jt(c^{\nom}_{i} + \lamVec^T \s - \lamVec^T \s^{\nom})}] \\
    &= \exp(jt(c^{\nom}_i - \lamVec^T\s^{\nom})) \mathbb{E}[e^{jt\lamVec^T\s}] \\
    &= \exp(jt(c^{\nom}_i - \lamVec^T\s^{\nom})) \phi_{\s}(t\lamVec) \\
    &= \exp(jt(c^{\nom}_i - \lamVec^T\s^{\nom})) \exp(j\lamVec^T\s^{\nom} - \frac{1}{2}t^2\lamVec^T \Sigs\lamVec) \\
    &= \exp(jtc^{\nom}_i - jt\lamVec^T\s^{\nom} + j\lamVec^T\s^{\nom} - \frac{1}{2}t^2\lamVec^T \Sigs \lamVec) \\
    &= \exp(jtc^{\nom}_i -\frac{1}{2}t^2\lamVec^T \Sigs \lamVec) \label{eq:crit_perf_char_eqn}
\end{align}

We can see from \eqref{eq:crit_perf_char_eqn} that it is the characteristic function of a normal distribution defined as

\[
    c_i \in N(c^{\nom}_{i}, \lamVec^T \Sigs \lamVec)
\]

with a mean $c^{\nom}_i$ and a variance $\lamVec^T \Sigs \lamVec$. Given that the variance is $\lamVec^T \Sigs \lamVec$ the standard deviation is simply

\[
    \sigma_{c_i} = \sqrt{\lamVec^T \Sigs \lamVec}
\]

We can determine the worst-case direction for our critical performance by solving
\[
    c^{\wc}_{i} = c^{\nom}_{i} + \Phi^{-1}(\rho)\sigma_{c_i}
\]
where $c^{\nom}_{i}$ is the nominal or mean critical performance value, $\Phi^{-1}$ is the inverse standard normal CDF $(\mu=0, \sigma=1)$, $\sigma_{c_i}$ is the standard deviation of the critical performance.
